# Supplementary material for: Double Control Variates for Gradient Estimation in Discrete Latent Variable Models
Source: arXiv:2111.05300 source file (2022-06-04)
Supplement: Supplementary file 1 [file supplement.tex]

\documentclass[twoside]{article}

\usepackage{aistats2022}

\usepackage{hyperref}
\usepackage{url}
\usepackage{algorithmic}
\usepackage{algorithm}
\usepackage{graphicx}
\usepackage{enumitem}
\usepackage{booktabs}

\usepackage{graphicx}

\providecommand{\definitionname}{Definition}
\providecommand{\assumptionname}{Assumption}
\providecommand{\lemmaname}{Lemma}
\providecommand{\propositionname}{Proposition}
\providecommand{\theoremname}{Theorem}

\begin{document}

\onecolumn
\aistatstitle{Supplementary Material\\
}

\input{tex/appendix}

\vfill

\end{document}
